# Supplementary material for: Hierarchical Composable Optimization of Web Pages
Source: arXiv:1110.0704 source file (2011-10-04)
Supplement: Supplementary file 1 [file Appendices.tex]

\appendix

\section{Layout HTML Example}\label{app: layout html}

%\parbox[b]{10cm}{
\begin{verbatim}
<html>
 <body>
  <table label="layout">
   <tr label="header" />
   <tr label="body">
    <td label="westRegtion" />
    <td label="centerRegtion">
     <table>
      <tr label="centerUpRegion">
       <td></td>
      </tr>
      <tr label="centerButtomRegion">
       <td></td>
      </tr>
     </table>
    </td>
    <td label="eastRegtion">
     <table>
      <tr label="East1Region">
       <td></td>
      </tr>
      <tr label="East2Region">
       <td></td>
      </tr>
      <tr label="East3Region">
       <td></td>
      </tr>
      <tr label="East4Region">
       <td></td>
      </tr>
     </table>
    </td>
   </tr>
  </table>
 </body>
</html>
\end{verbatim}

\section{POTL Example}\label{app: POTL file}

\begin{verbatim}
<layout label="MainPage">
 <apl:constraints id="MainPageConstraints">
  <region label="YahooHeader">
   <module label="YahooHeaderModule">
    <source label="YahooHeaderSource">
     <apl:operator id="yahooHeaderOperator" 
handler="YahooHeaderSearcherChain" />
    </source>
    <renderer label="YahooHaederRendererHandler" />
   </module>
  </region>
  <region label="YahooSitesRegion">
   <module label="YahooSitesModule">
    <source label="YahooSiteSource">
     <apl:constraints id="YahooSitesConstraints">
     <!-- Mapping 18 items out of 30 to 18 positions -->
       <apl:map id="YahooSiteMap" 
handler="SiteSelectorSearcherChain">
        <apl:operator id="yahooSiteOperator" 
handler="YahooSiteSearcherChain">
         <property key="number of regions" value="18" />
         <property key="number of items" value="30" />
         </apl:operator>
          </apl:map>
           <apl:constraint id="YahooSiteConstraint1">
            <![CDATA[function isValid(query, executionMap) {
            // Mail and messenger sites can't be in 
            // consecutive positions.
            }]]>
           </apl:constraint>
           <apl:constraint id="YahooSiteConstraint2">
            <![CDATA[function isValid(query, executionMap) {
            // If travel site is included then 
            // weather is included as well.
            }]]>
           </apl:constraint>
           <apl:constraint id="YahooSiteConstraint3">
            <![CDATA[function isValid(query, executionMap) {
            // Mail is always mapped to the first position.
            }]]>
           </apl:constraint>
          </apl:constraints>
         </source>
         <renderer label="YahooSiteRendererHandler" />
        </module>
       </region>
       <region label="TodayRegion">
        <module label="TodayModule">
         <source label="TodaySource">
          <apl:constraints id="TodayConstraints">
          <!-- Mapping 4 items out of 500 to 4 place holders -->
           <apl:map id="TodayMap" 
handler="HotItemSearcherChain">
            <region label="news1">
             <apl:position id="news1" />
            </region>
            <region label="News2">
             <apl:position id="news2" />
            </region>
            <region label="News3">
             <apl:position id="news3" />
            </region>
            <region label="News4">
             <apl:position id="news4" />
            </region>
            <apl:operator id="NewsOperator" 
handler="NewsSearcherChain">
           </apl:operator>
          </apl:map>
          <apl:constraint id="TodayConstraint1">
           <![CDATA[function isValid(query, executionMap) {
                    // No more than 2 sport news items.
                    }]]>
          </apl:constraint>
          <apl:constraint id="TodayConstraint2">
           <![CDATA[function isValid(query, executionMap) {
           // At least one geo local news item (relates to the geographical 
           // location of the user).
           }]]>
          </apl:constraint>
          <apl:constraint id="TodayConstraint3">
           <![CDATA[function isValid(query, executionMap) {
           // The first news item must be less than 2 hours old.
           }]]>
          </apl:constraint>
         </apl:constraints>
        </source>
        <renderer label="TodayRendererHandler" />
       </module>
      </region>
      <region label="TrendingNowRegion">
       <module label="TrendingNowModule">
        <source label="TrendingNowSource">
         <apl:constraints id="TrendingNowConstraints">
         <!-- Mapping 10 items out of 300 to 10 place holders -->
           <apl:map id="TrendingNowMap" 
handler="InorderMapSearcherChain">
            <apl:operator id="TrendingNowOperator" 
handler="TrendingNowSearcherChain">
             <property key="number of regions" value="10" />
             <property key="number of items" value="300" />
            </apl:operator>
           </apl:map>
           <apl:constraint id="No more of 2 trends of the same category contencuse">
            <![CDATA[function isValid(query, executionMap) {
             // No more than 3 celeb related trends.
            }]]>
           </apl:constraint>
           <apl:constraint id="long queries in the five last positions">
            <![CDATA[function isValid(query, executionMap) {
            // Trends with more than 2 words can't 
            // be placed in the same row
            }]]>
           </apl:constraint>
          </apl:constraints>
         </source>
         <renderer label="TrendingNowRendererHandler" />
        </module>
      </region>
      <region label="DisplayAds">
       <module label="DisplayAdsModule">
        <source label="DisplayAdsSource">
         <apl:operator id="DisplayAdsOperator" 
handler="DisplayAdsSearcherChain" />
        </source>
        <renderer label="DisplayAdsRendererHandler" />
       </module>
      </region>
      <region label="VeritcalHeadlines">
       <module label="VeritcalHeadlinesModule">
        <source label="VeritcalHeadlinesSource">
         <apl:operator id="VeritcalHeadlinesOperator" handler="VeritcalHeadlinesSearcherChain" />
        </source>
        <renderer label="VeritcalHeadlinesRendererHandler" />
       </module>
      </region>
      <region label="LatestVideo">
       <module label="LatestVideoModule">
        <source label="LatestVideoSource">
         <apl:operator id="LatestVideoOperator" 
handler="LatestVideoSearcherChain" />
        </source>
        <renderer label="LatestVideoRendererHandler" />
       </module>
      </region>
      <region label="YahooVertical">
       <module label="YahooVerticalModule">
        <source label="YahooVerticalSource">
         <apl:choice id="ImageColorChoice">
          <apl:alternative id="vertical1Alternativ">
           <apl:operator id="vertical1" 
handler="VerticalInfoSearchChain">
            <proprty key="verticalId" value="cars" />
           </apl:operator>
          </apl:alternative>
          <apl:alternative id="vertical2Alternativ">
           <apl:operator id="vertical2" 
handler="VerticalInfoSearchChain">
            <proprty key="verticalId" value="jobs" />
           </apl:operator>
          </apl:alternative>
          <apl:alternative id="vertical3Alternativ">
           <apl:operator id="vertical3" 
handler="VerticalInfoSearchChain">
            <proprty key="verticalId" value="games" />
           </apl:operator>
          </apl:alternative>
         </apl:choice>
        </source>
        <renderer label="YahooVerticalRendererHandler" />
       </module>
      </region>
     </apl:constraints>
    </layout>
   </apl:template>
\end{verbatim}
